# Supplementary material for: DBL: Efficient Reachability Queries on Dynamic Graphs (Complete Version)
Source: arXiv:2101.09441 source file (2021-04-15)
Supplement: Supplementary file 1 [file appendix.tex]

\section{Appendix}\label{sec:appendix}

\begin{table*}[t]
	\centering
	\caption{Query time for vertex pairs with different distances(ms)}
	\vspace{-1em}
	\label{tab:query-distance}
	\begin{tabular}{cccccc}
		\hline
		Dataset  & 2-hop & 4-hop & 6-hop & 8-hop & unreachable \\
		\hline
		LJ&6.99(99.98)&4.80(100)&3.10(100)&12.17(99.75)&59.97(99.02)\\
		Web&13.42(98.36)&5.70(99.48)&3.87(100)&3.66(100)&30.45(97.03)\\
		Email&4.42(98.83)&4.10(98.83)&2.67(99.73)&3.17(99.29)&4.77(99.09)\\
		Wiki&13.84(99.85)&4.11(100)&28.33(99.05)&--&45.92(99.60)\\
		Pokec&2.70(100)&4.49(100)&3.40(100)&3.69(99.79)&17.90(99.72)\\
		BerkStan&11.1(97.81)&1.99(99.98)&5.04(99.30)&17.82(97.22)&322.05(90.12)\\
		Twitter&9.36(99.99)&9.18(99.86)&34.26(98.91)&21.19(99.61)&87.46(96.64)\\
		Reddit&4.00(100)&10.54(99.93)&32.25(98.77)&24.72(98.88)&25.68(99.56)\\
		\hline
	\end{tabular}
	\vspace{-1em}
\end{table*}

\begin{table}[t]
	\centering
	\caption{Query time (ms) for different centrality heuristics. A=$\max(|Pre(\cdot)|,|Suc(\cdot|))$; B=$\min(|Pre(\cdot)|,|Suc(\cdot|))$;
		C=$|Pre(\cdot)|+|Suc(\cdot)|$; \textcolor{red}{D is the betweenness centrality;} ours=$|Pre(\cdot)|\cdot|Suc(\cdot)|$}
		\vspace{-1em}
	\label{tab:landmark-rank}
	\begin{tabular}{cccccc}
		\hline
		Dataset  & A & B & C & D & ours  \\
		\hline
		LJ        &125.10      &127.84    &105.88     &113.34     &108.51  \\
		Web       &202.16      &144.13    &142.16     &140.79     &139.64     \\
		Email     &37.02       &37.01     &36.14      &38.53      &36.38   \\
		Wiki      &156.21      &159.74    &153.66     &155.45     &157.12          \\
		Pokec     &37.69       &64.57     &36.96      &50.66      &34.78   \\
		BerkStan  &1890        &6002      &1883       &1252       &1590  \\
		Twitter   &719.31      &849.78    &685.31     &727.59     &693.71  \\
		Reddit    &99.21       &65.06     &62.68      &69.62      &60.48  \\
		\hline
	\end{tabular}
	\vspace{-1em}
\end{table}

\subsection{BL Label Node Selection}\label{sec:app:leaf}

In the main body of this paper, we restrict the leaf nodes to be the ones with either zero in-degree or zero out-degree.
Nevertheless, our proposed method does not require such a restriction and could potentially select any vertex with low centrality as a leaf node.
Following the approach for which we select \dl label nodes,
we use  $M(u) = |Pre(u)| \cdot |Suc(u)|$ to approximate the centrality of vertex $u$
and select vertex $u$ as a \bl label node if $M(u) \leq r$ where $r$ is a tunning parameter. Assigning $r=0$ produces the special case presented in the main body of this paper. The algorithms for query processing as well as index update of the new \bl label remains unchanged.
Figure~\ref{fig:bl-degree} shows the query performance of \sol when we vary the threshold $r$.
With a higher $r$, more vertices are selected as the leaf nodes, which should theoretically improve the query processing efficiency.
However, since we employ the hash function for \bl label, more leaf nodes lead to higher collision rates. This explains why we don't observe a significant improvement in query performance.

\begin{figure}[b]
	\centering
    \vspace{-2em}
	\includegraphics[width=0.4\textwidth]{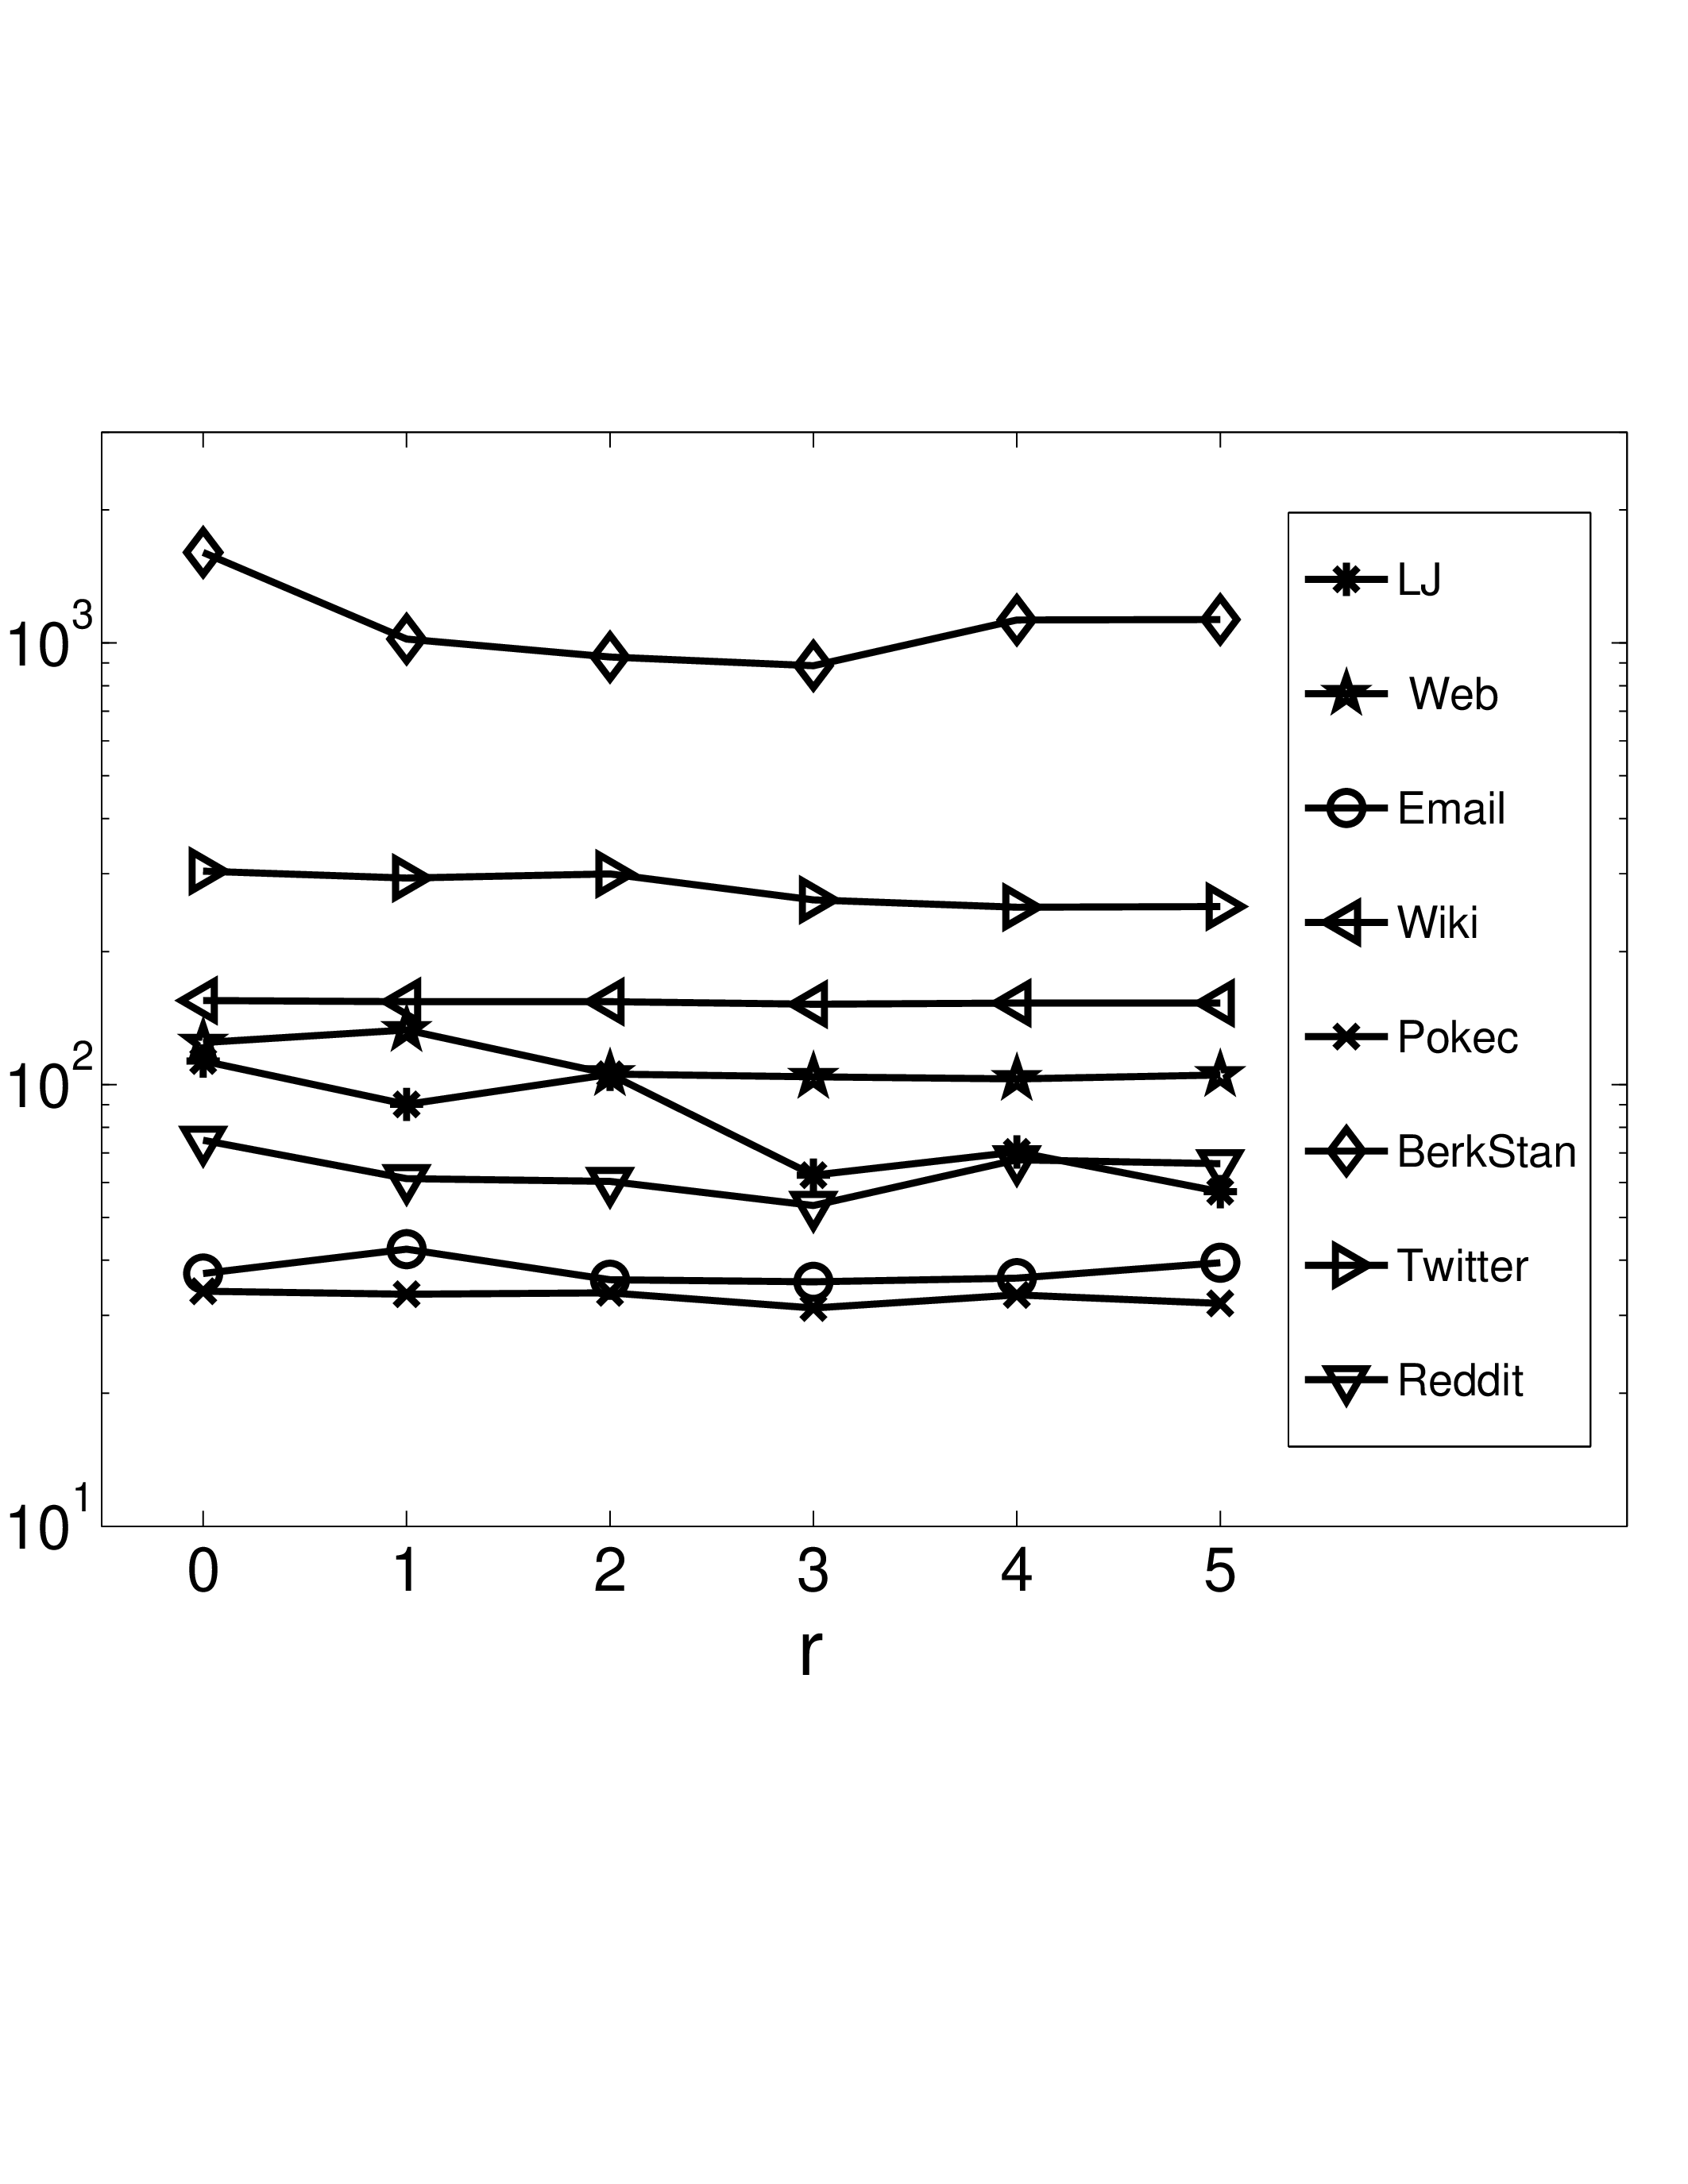}
    \vspace{-1em}
	\caption{\bl label node selection}
	\label{fig:bl-degree}
    \vspace{-1em}
\end{figure}

\subsection{Profiling of the Centrality Heuristic}\label{sec:landmark-rank}

Both \dl and \bl select the label nodes by heuristically approximating the centrality of a vertex $u$ as $M(u) = |Pre(u)| \cdot |Suc(u)|$.
In the appendix, we evaluate different heuristic methods for centrality approximation. The results are shown in Table~\ref{tab:landmark-rank}. Overall, our adopted heuristic ($|Pre(u)| \cdot |Suc(u)|$) achieves the performance. For Email and Wiki, all the methods share a similar performance. $|Pre(\cdot)|+|Suc(\cdot)|$ and $|Pre(\cdot)|\cdot|Suc(\cdot)|$ get a better performance in other datasets. Finally, $|Pre(\cdot)|+|Suc(\cdot)|$ and $|Pre(\cdot)|\cdot|Suc(\cdot)|$ deliver similar performance for most datasets and the latter is superior in the Berkstan dataset.
Thus, we adopt $|Pre(\cdot)|\cdot|Suc(\cdot)|$ for approximating the centrality. \textcolor{red}{It needs to mention that, although the betweenness centrality get a medium overall performance, it shows the best performance in BerkStan dataset.}

\subsection{Update for Real World Graph}\label{index-update}

We report additional results on real-world dynamic graphs: sx-stackoverflow (SX) and wiki-talk-temporal (WTALK) from SNAP \cite{snapnets}. WTALK consists of 1,140,149 vertices and 7,833,140 edges and SX is a much larger graph which has 2,601,977 vertices and 63,497,050 edges.
As each edge has a timestamp, we order the edges according to their timestamps and run a sliding window which contains the first 50\% of edges in each dataset to maintain a temporal graph that gets updated once the window slides. Table~\ref{tab:scc-update-sx} presents the results for SX and WTALK.
We report the number of \dagg updates and the running time of processing edge updates after every 10000 window slides. As both \ip and \tol can't handle real-world update, we use \dgr as baseline instead. The results have shown that the number of \dagg updates is significant and cannot be ignored. For example, there are 2471 and 3844 \dagg updates for 50000 window slides. However, it takes hours to process the updates. In comparison, \sol completes the index update in 48.71 and 2.81 seconds, which shows that our proposed index update approaches are sufficient to handle real-world dynamic graph updates efficiently.

\begin{table}[t]
	\centering
	\caption{Profiling of the real-world graph updates}
		\vspace{-1em}
	\label{tab:scc-update-sx}
    \small
	\begin{tabular}{|c|ccc|ccc|}
		\hline
		& \multicolumn{3}{c|}{SX} & \multicolumn{3}{c|}{WTALK} \\
		\hline
		\multirow{2}{*}{Slides}  & \dgr & \sol & \dagg  & \dgr & \sol & \dagg \\
		& (s) & (s) & updates & (s) & (s) & updates \\
		\hline
		10000&13417 &21.65 &469 &1912 &0.93 &691 \\
		20000&27434 &28.42 &939  &4021 &1.39 &1378\\
		30000&46420 &35.17 &1365 &6801 &1.86 &2013 \\
		40000&66246 &40.94 &1838  &10967 &2.35 &2810  \\
		50000&89846 &48.71 &2471  &14036 &2.81 &3844  \\
		60000&110312 &55.51 &3054  &16907 &3.24 &4640  \\
		70000&131628 &62.28 &3534  &20005 &3.66 &5571  \\
		80000&154159 &68.13 &4012 & 23151 &4.08 &6451  \\
		\hline
	\end{tabular}
	\vspace{-1em}
\end{table}

\subsection{Vary Query Hop Distance}\label{query-distance}

To further validate the effectiveness of \sol, we evaluate the query performance of the node pairs in different distances.
For each scenario, one hundred thousand queries are generated in a totally random manner. Table~\ref{tab:query-distance} shows the query time. The number in bracket is the percentage of the queries directly answered by \dl and \bl labels. The dash line means that there are not enough queries for that particular distance setup.
In fact, for pairs of vertices that are 2-hops away, 4-hops away or 6-hops away, the query performance will make a difference only when the \bfs procedures are required. Generally, a longer distance tends to cost a larger overhead as the \bfs procedure will need more time to traversal the graph. However, the percentage of queries that answered by label will also have a great impact on the total query time which could explain the fluctuation in the query performance.

%\subsection{Query Error Ratio without DAG Update}\label{query-distance}
%
%
%One of the most important contribution of our work is that our method is \dagg free. Thus, we compute how much error it will incur if \dgr don't maintain the \dagg. As the edge insertion is a much more common operation in graph update, we insert 100 to 400 edges respectively. Every edge update are followed by ten random queries. For most of the dataset, the query error ratio is low. as nearly 80 percent of the nodes are in the biggest \scc, thus, edge insertion could hardly alter the \dagg structure.
